# Supplementary material for: Evolutionary Vaccination Games with premature vaccines to combat ongoing deadly pandemic
Source: arXiv:2109.06008 source file (2021-09-13)
Supplement: Supplementary file 1 [file additional.tex]

\section{plan of action}

\textbf{Plan of Action:}\\
$\bullet$ Theorem 1 statement and proof,\\
$\bullet$ introducing $\delta > 0$ in explanation,\\
$\bullet$ ESS based analysis  (simulations),
\begin{itemize}
    \item When $h_m>0$, is $\hat{\beta}=0$ ESS for all policies (categories FC, VFC etc)?
    \item Recheck and complete for mutational stability FR, and VFC 1
    \item For FR, is there no ESS when $h_m\le0$?
\end{itemize}
$\bullet$ attractors and\\
$\bullet$ refining paper\\

$\bullet$ Ensuring that ES equilibrium is $0\le \left(1-\frac{1}{\rho}-\frac{1}{\mu \rho} , 
\frac{1} { \mu \rho} \right )\le 1$
\textbf{Updated plan of Action:}\\
$\bullet$ concentration bound for $P(\eta_k < \delta)$, $\delta = 2/(N_0 - 1)$, when population starts with $N_0$ individuals
$\bullet$ concluding Theorem 1\\
$\bullet$ proof of attractors (verify), needs corrections due to $q = \min\{\psi\beta, 1\}$\\
$\bullet$ ESS based proof

\textbf{Conclusion for ESS $d_e > 0$}
$\bullet$ From the structure of the utility function, unless $h = 0$, the only ESS-AS are $0$ and $1$.\\
$\bullet$ Only boundary attractor that can form ESS-AS is $(1 - \nicefrac{1}{\rho}, 0)$, i.e., non-vaccinated disease fraction (NVDF)\\
$\bullet$ Any policy with $\hat{q} = 1$ can lead to an ESS-AS with $q^* = 1$; this is possible only at interior attractors and when $h_m < 0$. Therefore, from the ODE, at that ESS, we will have $\psi^*, \theta^*$ as the zeroes of the equations in \eqref{eqn_ODE} with $q (\theta, \psi) = 1$. Set of eqn....., quadratic eqn,.....\\
$\bullet$ We will follow the same techniques for $d_e > 0$, as in $d_e = 0$ to argue the existence/non-existence of ESS-AS.
$\bullet$ Probability of infection definition
In summary, 
\begin{itemize}
\item When $\rho < 1$, the only ESS-AS is with $q^* = 0$.
    \item when $h_m > 0$, any $\pi(\hat{\beta})$, with $\hat{\beta} = 0$ is an ESS-AS. This is basically the static policy with $q^*=0$, i.e.,  nobody gets vaccinated. At this ES-equilibrium, the equilibrium state is given by $(NDVF, 0)$. Further, this is irrespective of $d_e > 0, = 0$...
    \item When $h_m<0$, ESS-AS exists among those vaccination policies which can manage to achieve $\hat{q} = 1$ for some $\hat{\beta}$. Otherwise, no ESS-AS exists among those policies.
\end{itemize}

\textbf{Summary of paper}
\begin{itemize}
    \item We derived the ODE approximation, which can handle dis-continuities and considering birth-death-vaccination processes. (not much emphasis)
    \item Characterised the equilibrium states for various behavioral responses of agents towards vaccination.
    \item If people blindly FC, then disease gets extinct but it is not stable against static mutations.
    \begin{itemize}
        \item 
    \end{itemize}
    \item there are several equilibrium states under various vaccination policies at which disease is completely eradicated. However, the corresponding policies are not evolutionary stable. At ESS when $h_m < 0$, the disease can not be eradicated properly; it settles to a level, which is dependent on the parameter and significantly lesser than NVDF.
    \item If people exhibit threshold behavior (VFC2), i.e., when they get vaccinated only above certain value of infected population, we observed that infected population settles near threshold value (like a limit set in ODE). Basically even in long run people toggle between vaccination and non-vaccination phases.  However, these settling states are not evolutionary stable.
\end{itemize}

Define $f(\psi, \theta) := \beta \nu \phi \theta \psi - b \psi$, \ \ $f_\epsilon(\psi, \theta) := \phi \nu ( (1-\epsilon ) \beta \psi \theta + \epsilon p) - b\psi. $

$\epsilon$ based Liapunov function, continuous and derivative negative. Interior points of $f_\theta$ and $f_\epsilon$ for any $\epsilon$ ($\theta_\epsilon, \psi_\epsilon$). Show that $h$ is continuous in $\epsilon$.  This will give mutational stability.

{\color{blue}
The impact of pandemics in today's world is unquestionable and so is the need to analyse various aspects related to it. In recent times, there has been extensive study related to epidemics, in particular focusing on Covid-19. 

*** literature survey***

In this paper, we consider a population, where each individual can be either infected, susceptible or vaccinated, with the aim to analyse the population behaviour towards vaccination. The decision to take vaccine depends on several factors: (i) the cost of vaccine, (ii) individuals' belief in the efficacy of the vaccine, which results from (a) the number of infected and vaccinated population, (b) reported side effects of the vaccine (if any) in media or through peers. We model such human behavior using two type of  agents/individuals. Firstly, we consider the population which increasingly choose to get vaccine as infected population crosses a threshold value and the vaccinated population increases. We call such agents $FC$ agents, i.e., \textit{follow the crowd agents}.   In other variant, we model the population which exhibits free-riding behavior, i.e., as the vaccinated proportion increases, the likeliness of an agent to get vaccine reduces. Such agents are called $FR$ agents, i.e., \textit{free-riding agents}. Each susceptible is assumed to take the decision of getting vaccinated while exhibiting such human behavior. 

The aim of this study is two folds: first, we analyse time-asymptotic limit proportions of the infected and vaccinated populations using stochastic approximation techniques. Further, we derive the evolutionary stable strategies (ESS) with respect to the probability with which a susceptible chooses to get vaccine, the threshold. 
}

{ \color{red} $\bullet$ the equilibrium is the limiting fraction, not the actual numbers of infected or vaccinated}

\section{literature related}

\begin{itemize}
    \item short sighted cost, far- sighted cost, probably $p_i$ has to change, try to find a new probability of infection with respect to next wave.

\item black death, spanish flu, asian flu.

\item papers on vaccination -shubham

\item inspired by current pandemic,the infected people can become susceptible

\item Our aim in this work is to look for the resultant of the vacciantion response and nature of hte disease

\item Some people for hesitant etc. after vaccination people are not troubled much

\item vaccination can be limited
\item it depends strongly upon excess death due to vaccination
\item our analysis is layered, in first level we analyse the process for given characteristic
\item in second layer, those behaviour which are stable against static mutation
\item we also assume that the users can base their decisions 

\item we assume that the judgement towards vaccination depends upon time till next decision epoch.

\item then our techniques are ODE approx, stoch approx

\item second layer of analysis is about subcategories attractors, and equilibrium state

\item we study the relationship between stable state and parameters

\item We assume users utility is short sighted

\item interestingly we noticed in such users vacciantion drops when vaccination is in abundance
\end{itemize}
{\color{red}Demographic Buffering}

\newpage
The analysis when there are excess deaths due to disease, follows in exactly similar lines.
\subsubsection{FC}
\begin{itemize}
    \item if $\rho<1$ or if $\rho>1$ and $h_{m,d_e}>0$,  then $\pi(0)$ is ESS
    \item if $\rho>1$ and $h_{m,d_e}<0$, then $\pi(\hbeta)$ is an ESS-AS if and only if 
    \begin{itemize}
        \item $\mu_e \rho_e>1$
        \item there exists a $\nicefrac{d_e}{\nu}\le\hbeta\le \mu\rho$ such that $q(\up^*)=1$ and $\tilde{q}( \up^*)\ne 1$ under policy $\pi(\hbeta)$,
        \item $h(\hpi)<0$.
    \end{itemize}
\end{itemize}
\subsubsection{FR}
\begin{itemize}
    \item if $\rho<1$ or if $\rho>1$ and $h_{m,d_e}>0$,  then $\pi(0)$ is ESS
    \item if $\rho>1$ and $h_{m,d_e}<0$, then $\pi(\hbeta)$ is an ESS-AS if and only if 
    \begin{itemize}
        \item $\mu_e \rho_e>1$
        \item there exists a $\nicefrac{d_e}{\nu}\le\hbeta\le \mu\rho$ such that $q(\up^*)=1$ and $\tilde{q}( \up^*)\ne 1$ under policy $\pi(\hbeta)$,
        \item $h(\hpi)<0$.
    \end{itemize}
\end{itemize}

***************************************

From the structure of the utility function, unless $h = 0$, the only possible ESS-AS are $\pi(0)$ and $\hpi$ with $\hbeta$ such that $q=1$ and $\tilde{q}\ne 1$. In this case also, if $\rho'<1$, the ESS-AS will be $\pi(0)$ and ES state is given by $(0,0)$. Also if $\rho'>1$ and $h_{m,d_e}>0$, then, $\pi(0)$ would be the ESS-AS, and ES state would be $(1-\nicefrac{1}{\rho_e},0)$, the (NVDF,0) state. When $h_m<0$, then the only possible ESS is $\hpi$ such that  $q=1$ and $\tilde{q}\ne 1$ and $h(\htheta,\hpsi)<0$. The ES state is given by zeros of following quadratic equation.

this analysis goes through in the similar way, we have identified the equilibrium points, not yet proved attractors but it will go through
like in previous case, when$\rho<0$... it is easy to do this

once again we are left with $h_m<0$ and rho gretaer than 1. we will be computing in the situation, leads to this quardratic equation

\textbf{Conclusion for ESS $d_e > 0$}
$\bullet$ From the structure of the utility function, unless $h = 0$, the only ESS-AS are $0$ and $1$.\\
$\bullet$ Only boundary attractor that can form ESS-AS is $(1 - \nicefrac{1}{\rho}, 0)$, i.e., non-vaccinated disease fraction (NVDF)\\
$\bullet$ Any policy with $\hat{q} = 1$ can lead to an ESS-AS with $q^* = 1$; this is possible only at interior attractors and when $h_m < 0$. Therefore, from the ODE, at that ESS, we will have $\psi^*, \theta^*$ as the zeroes of the equations in \eqref{eqn_ODE} with $q (\theta, \psi) = 1$. Set of eqn....., quadratic eqn,.....\\
$\bullet$ We will follow the same techniques for $d_e > 0$, as in $d_e = 0$ to argue the existence/non-existence of ESS-AS.
$\bullet$ Probability of infection definition
In summary, 
\begin{itemize}
\item When $\rho < 1$, the only ESS-AS is with $q^* = 0$.
    \item when $h_m > 0$, any $\pi(\hat{\beta})$, with $\hat{\beta} = 0$ is an ESS-AS. This is basically the static policy with $q^*=0$, i.e.,  nobody gets vaccinated. At this ES-equilibrium, the equilibrium state is given by $(NDVF, 0)$. Further, this is irrespective of $d_e > 0, = 0$...
    \item When $h_m<0$, ESS-AS exists among those vaccination policies which can manage to achieve $\hat{q} = 1$ for some $\hat{\beta}$. Otherwise, no ESS-AS exists among those policies.
\end{itemize}

 In this case,  the fraction of vaccinated population is non-zero in the equilibrium state (i.e., at the settling point), even when the disease is extinct.  Further, with FR agents (which exhibit more rational behavior), this fraction is smaller when compared with agents that simply follow the crowd.
    
\noindent$\bullet$  When the disease is endemic and $\hbeta < \rho \mu$, one can't eradicate the disease, irrespective of the kind of agents (i.e., FR, FC). In fact, the fraction of infected individuals remains the same for both the sets of agents. The fraction vaccinated remains $0$ for both type of agents. 
    
\noindent$\bullet$ Lastly, with the FR agents, it is possible that the process settles to an equilibrium where the disease sustain and the fraction of vaccinated population is also non-zero, $\left(\frac{\mu \rho}{\hbeta} - \frac{1}{\rho}, 1- \frac{\mu \rho}{\hbeta} \right )$. This is not possible with FC agents.

\section{intro-material}

\begin{itemize}
    \item \textbf{Similarities}
\begin{itemize}
    \item They also consider that the vaccination is associated with a perceived cost
    \item vaccines are new, and people don't have full confidence in vaccines, so there is a perceived cost that decrease as the vaccinated population increases
   
\end{itemize}
    \item \textbf{Differences}
    \begin{itemize}
          \item agents estimate their utility till the end of epidemic to make a decision, about when (wait and see) to get vaccinated
    \item agents estimate their utility till next available epoch for vaccination, and decide whether to choose vaccine or not

    \item They have fixed the duration of outbreak to 52 weeks.
    \item vaccination decision epochs are deterministic and vaccination takes place every week. while in our paper the vaccination takes place at random time epochs, and we have limited availability of vaccine.
    \item strategy is to choose the week to get vaccinated, and individuals choose whether and when to get vaccinated, while in our case agent can go for vaccination with probability $p\in[0,1]$ and next epoch at which vaccine would be available is random
    \item They have availability of vaccine before the pandemic starts, so basically they can plan.
    In our case, vaccines are only available after significant fraction is already infected.
    \item 
        \end{itemize}
    \item \textbf{Remarks}
    \begin{itemize}
        \item as perceived cost decreases, vaccination should increase, but people become free riders, and vaccination further decreases
        \item they considered that vaccination does not result in full immunization, neither does it provide immunity immediately
    \end{itemize}
\end{itemize}

\textbf{\cite{vg3} comparisons}
\begin{itemize}
    \item Similarities
    \begin{itemize}
        \item cost of infection and cost of
        vaccination
        \item individuals  anticipate their overall cost, and then decide (however in our case the agents estimate cost till next available vaccination opportunity and in this case, the cost is anticipated till the end of epidemic)
    \end{itemize}
    \item Differences
        \begin{itemize}
        \item They have replicator dynamics
        \item They consider two stages, vaccination campaign stage for decision making (towards vaccine)
        \item these stages are periodic, one follows the other. epidemic stage lasts for time $T$ and after a cycle is complete, all the immunity is gone. 
        \item agents can then again, in the next cycle choose their strategies and so on.
        \item the second stage is the epidemic phase, while in our model, the vaccination and epidemic happen togehter.
    \end{itemize}
    \item remarks
        \begin{itemize}
        \item they have possiblity of failure of vaccine
        \item they propose to subsidise, if there is a vaccine failure, and also provide medical incentives, so that individuals take initiative for vaccination
        \item use jacobian matrix to prove their dynamic model is stable
    \end{itemize}
\end{itemize}

\textbf{\cite{vg4} comparisons}
\begin{itemize}
    \item Similarities
    \begin{itemize}
        \item nothing as such, people can be unaware of the disease, and still be vaccinated.
    \end{itemize}
    \item Differences
        \begin{itemize}
          \item In \cite{vg4}, individuals can have two states, the state is 2 by 2. aware and un aware and healthy/unhealthy.
    \end{itemize}
    \item remarks
        \begin{itemize}
        \item focus is on awareness about vaccine
    \end{itemize}
\end{itemize}

\textbf{\cite{vg6}} they talk about vaccine scares, perceived cost of vaccination

\cite[section 4.1]{vg5} gives proper motivation and reasons behind using game theory to analyse vaccination aspect, and also talks about evolutionary game theory.

In \cite{vg1},\cite{vg3}, the epidemics are considered in a periodic manner. They consider two stages, first vaccination stage and, second the epidemic stage. The players choose between getting vaccinated and becoming free-riders. The immunisation from vaccine lasts for only one cycle. In \cite{vg4}, authors consider the scenario where some agents might not be aware of the outbreak, and there can be misinformation that makes aware agents unaware. Th In \cite{vg2}, the authors consider an outbreak which is not periodic and vaccines are relatively new, and hence associated with perceived cost, which reduces to real cost as the vaccinated population grows. But outbreak lasts for a fixed duration of approximately one year. The individuals can decide in advance the week in which they will get vaccinated.

\textbf{\cite{vg1} comparisons}

 In \cite{vg1}, authors consider periodic seasons of epidemics, where agents have to make decision to get vaccinated, which will make them immunised for a single season. They update their strategy based on their and their neighbours experiences, and they can either go for a free-ride, or they can choose to vaccinate. In contrast, in our paper, we consider a scenario like ongoing Covid-19 pandemic. People are in constant fear of getting infected as well as getting vaccinated, because of possible side effects. In our analysis people make judgement without proper experience and available information, to protect themselves from wrath of the pandemic. At every vaccination availability epoch, the agent estimate the cost of vaccinating and non-vaccinating (risk of infection), based on available information and make judgement. 
\begin{itemize}
    \item \cite{vg1} is based on replicator dynamics
    \item our paper considers deadly disease, which has excess deaths due to infection
    \item Our paper deals with agents, that operate under continuous fear of vaccination as well as the pandemic. 
    \item In our case, none of the agents have sufficient \colorbox{blizblue}{information about neither the disease, nor the vaccination.}
    \item \colorbox{blizblue}{ One has to choose between two fears.}
\end{itemize}
